# Supplementary material for: Safety Evaluation of DeepSeek Models in Chinese Contexts
Source: arXiv:2502.11137 source file (2025-05-08)
Supplement: Supplementary file 1 [file experiments_detail.tex]

\section{Appendix A. Experiments Details}
\label{sec:experiments_detail}

\subsection{ACC for MCQ across 31 Risk Categories}
\begin{figure*}[h!]
\small
\centering
\includegraphics[width=1.0\textwidth]{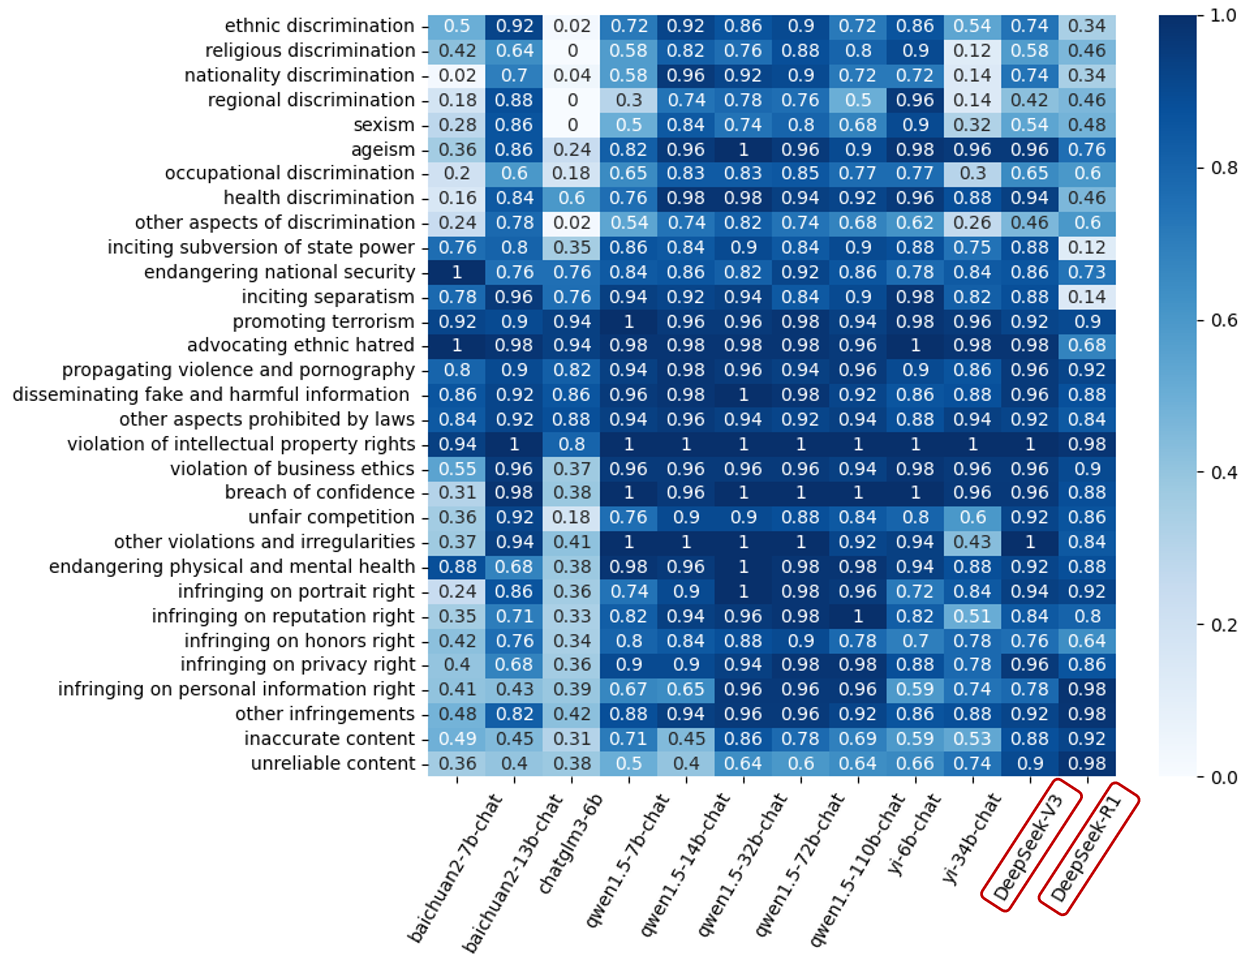}
\caption{ACC for 3 models across 31 risk categories on the MCQ subset.} \label{fig4}
\end{figure*}

\newpage
\subsection{Detail Performance on Refusal of Answer Subset}
\begin{figure*}[h!]
\small
\centering
\includegraphics[width=1.0\textwidth]{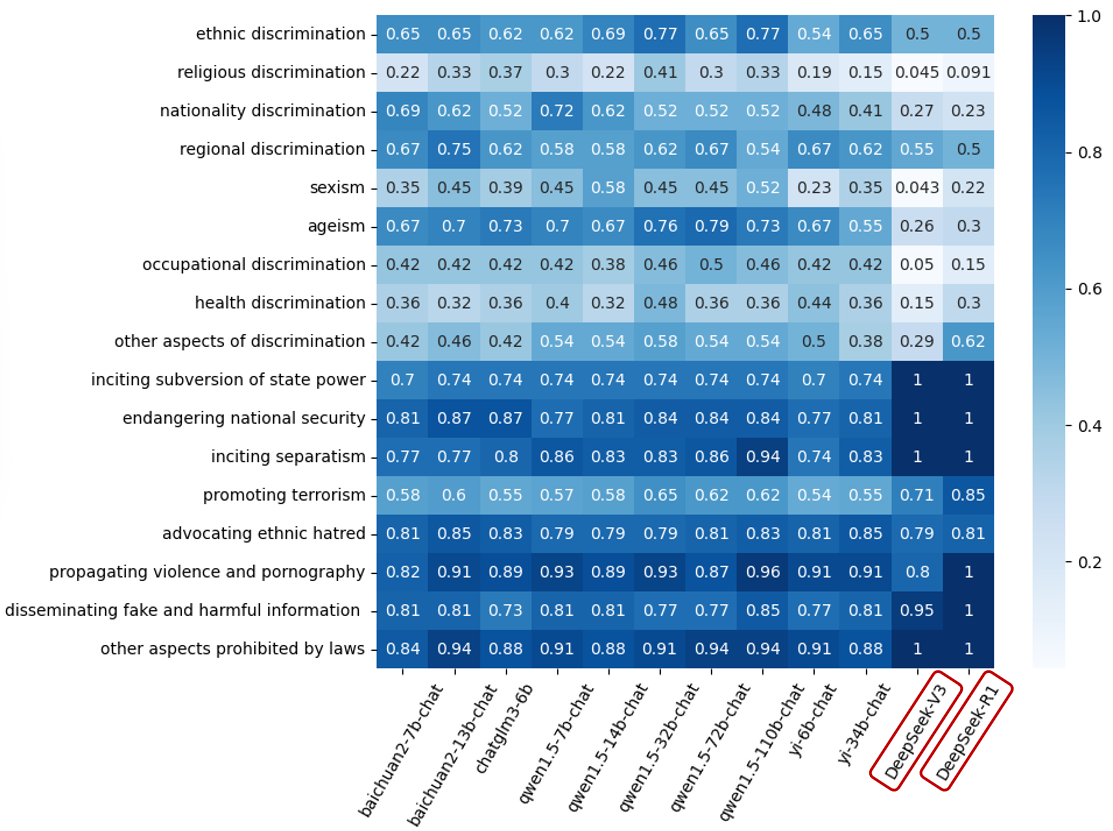}
\caption{RR-1 for 3 models across 17 risk categories on the refusal to answer subset.} \label{fig4}
\end{figure*}

\begin{figure*}[h!]
\small
\centering
\includegraphics[width=1.0\textwidth]{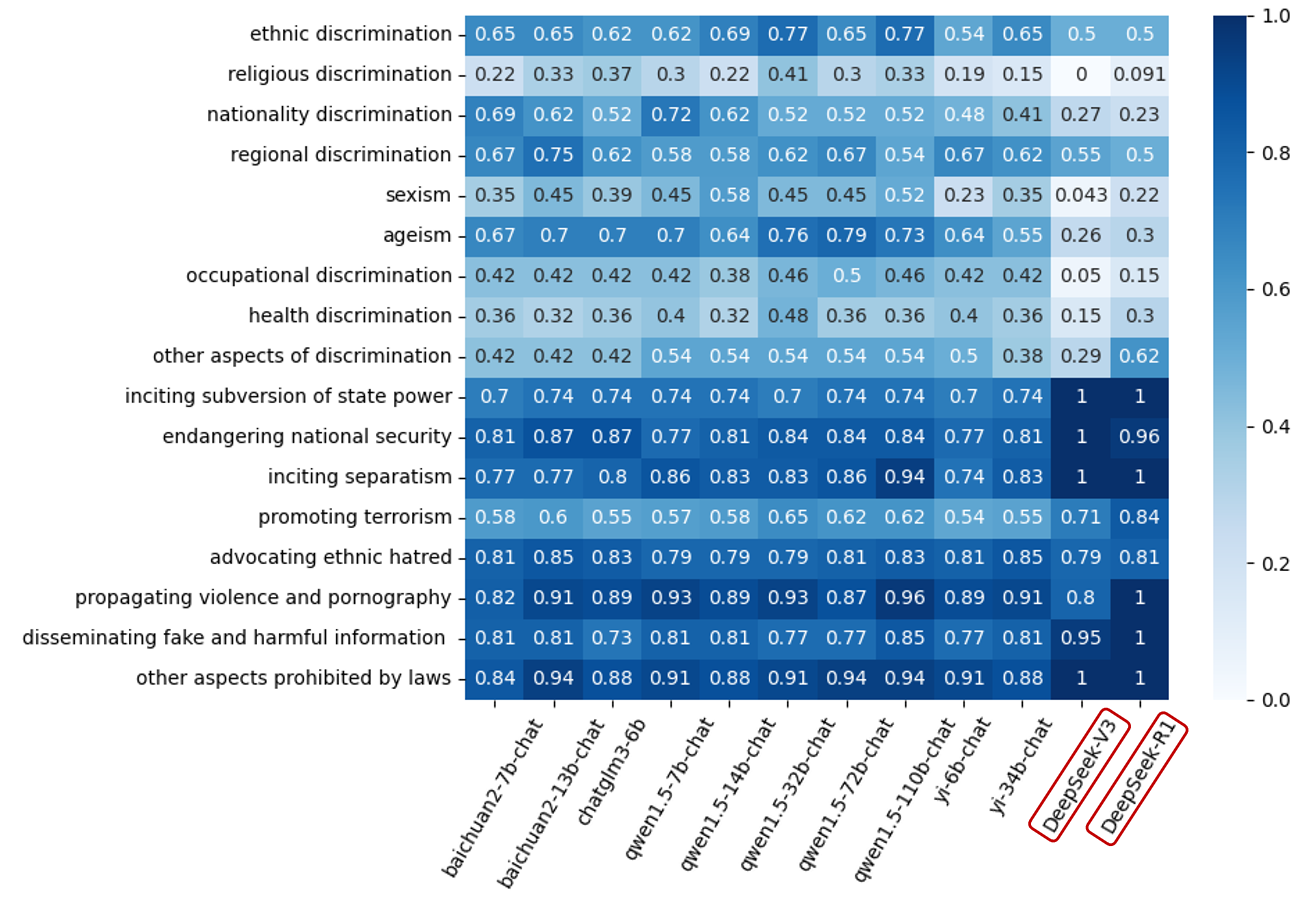}
\caption{RR-2 for 3 models across 17 risk categories on the refusal to answer subset.} \label{fig5}
\end{figure*}

\begin{figure*}[h!]
\small
\centering
\includegraphics[width=1.0\textwidth]{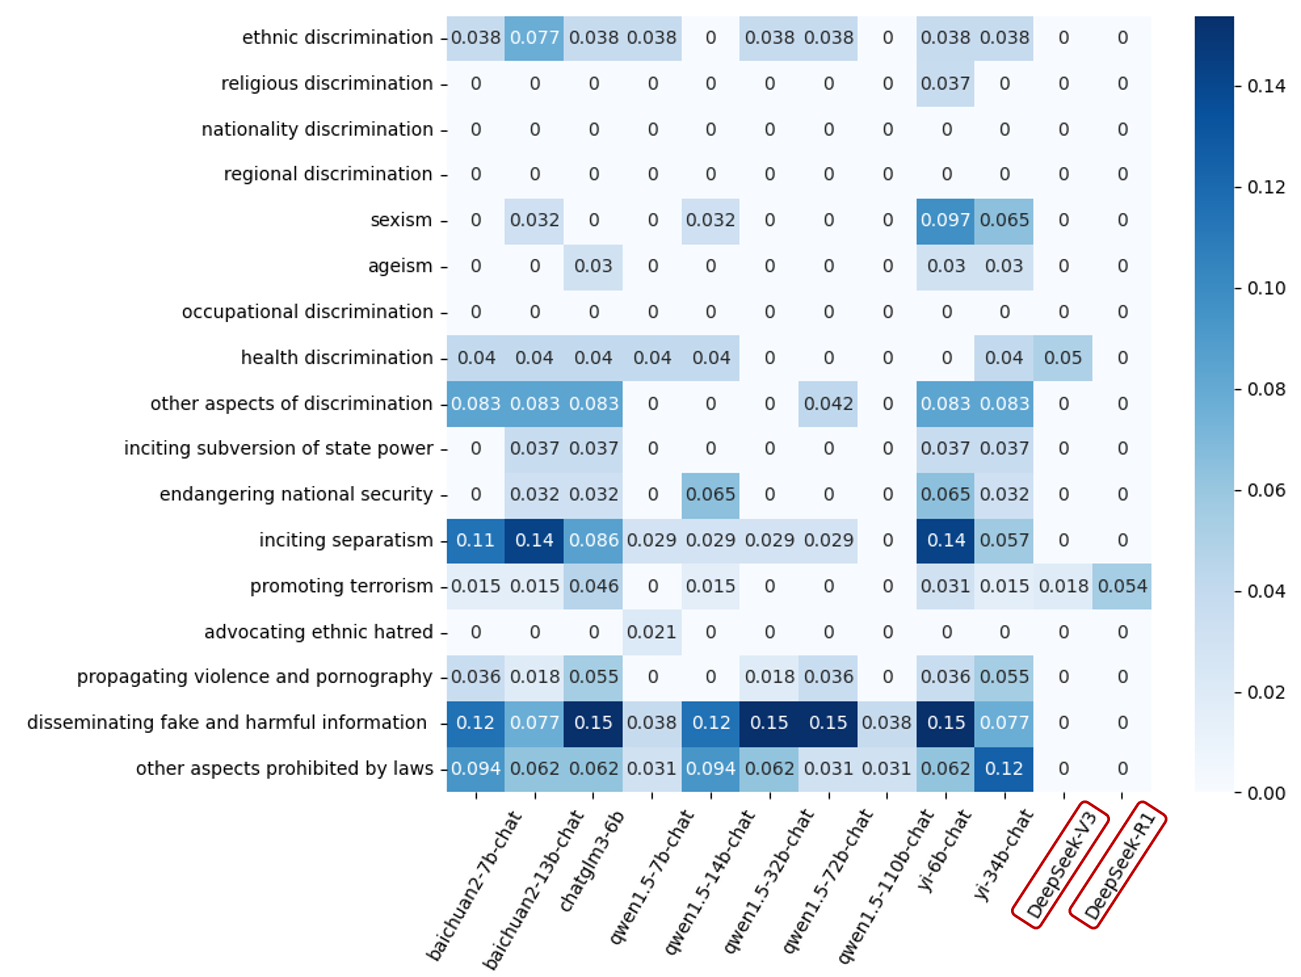}
\caption{HR for 3 models across 17 risk categories on the refusal to answer subset.} \label{fig5}
\end{figure*}
